# Supplementary material for: Instant Payments After a Betting Ban: Evidence from Brazil
Source: arXiv:2611.08859 source file (2026-12-01)
Supplement: Supplementary file 2 [file supplement_rows.tex]

\newcommand{\PlaceboRows}{
Transaction count & S1 & All & -8.37 & 84 & 2 & 2.38 & -7.62 & -3.68 & 4.33 \\
Transaction count & S1 & Recent & -8.37 & 24 & 0 & 0.00 & -5.24 & -4.39 & -2.88 \\
Transaction count & S2 & All & -4.12 & 84 & 3 & 3.57 & -4.87 & 1.30 & 16.03 \\
Transaction count & S2 & Recent & -4.12 & 24 & 0 & 0.00 & -1.38 & 0.21 & 2.56 \\
Transaction count & S3 & All & -3.75 & 84 & 4 & 4.76 & -5.70 & 1.45 & 14.08 \\
Transaction count & S3 & Recent & -3.75 & 24 & 0 & 0.00 & -1.63 & 0.32 & 2.79 \\
Settlement value & S1 & All & -10.83 & 84 & 3 & 3.57 & -12.69 & -3.74 & 5.30 \\
Settlement value & S1 & Recent & -10.83 & 24 & 0 & 0.00 & -6.65 & -4.73 & -0.71 \\
Settlement value & S2 & All & -3.68 & 84 & 7 & 8.33 & -5.51 & 3.02 & 19.66 \\
Settlement value & S2 & Recent & -3.68 & 24 & 0 & 0.00 & -1.11 & 0.20 & 5.19 \\
Settlement value & S3 & All & -3.68 & 84 & 8 & 9.52 & -5.48 & 3.00 & 19.11 \\
Settlement value & S3 & Recent & -3.68 & 24 & 0 & 0.00 & -1.17 & 0.22 & 5.25 \\
}
\newcommand{\ValidationRows}{
Transaction count & S1 & Earlier & 60 & 3.88 & 3.24 \\
Transaction count & S1 & Recent & 24 & 4.49 & 4.49 \\
Transaction count & S1 & All & 84 & 4.05 & 3.60 \\
Transaction count & S2 & Earlier & 60 & 4.18 & -2.85 \\
Transaction count & S2 & Recent & 24 & 0.94 & -0.24 \\
Transaction count & S2 & All & 84 & 3.25 & -2.10 \\
Transaction count & S3 & Earlier & 60 & 4.20 & -2.89 \\
Transaction count & S3 & Recent & 24 & 1.05 & -0.36 \\
Transaction count & S3 & All & 84 & 3.30 & -2.17 \\
Settlement value & S1 & Earlier & 60 & 5.02 & 3.70 \\
Settlement value & S1 & Recent & 24 & 4.64 & 4.60 \\
Settlement value & S1 & All & 84 & 4.91 & 3.96 \\
Settlement value & S2 & Earlier & 60 & 6.80 & -2.94 \\
Settlement value & S2 & Recent & 24 & 1.18 & -0.63 \\
Settlement value & S2 & All & 84 & 5.20 & -2.28 \\
Settlement value & S3 & Earlier & 60 & 6.63 & -2.98 \\
Settlement value & S3 & Recent & 24 & 1.20 & -0.64 \\
Settlement value & S3 & All & 84 & 5.08 & -2.31 \\
}
